# Supplementary material for: Deep Learning Models for Physical Layer Communications
Source: arXiv:2502.04895 source file (2025-02-07)
Supplement: Supplementary file 1 [file appendix_part_1.tex]

\chapter{Appendix}
\label{sec:appendix}

\section{Theoretical..}
\label{sec:appendix_part_1}
In ..
